# Supplementary material for: ChainedFilter: Combining Membership Filters by Chain Rule
Source: arXiv:2308.13632 source file (2023-08-25)
Supplement: Supplementary file 1 [file appendix.tex]

\begin{appendices}
\label{sec:appendix}
\section{1}
13
\end{appendices}
